# Supplementary material for: Neural Graphics Texture Compression Supporting Random Access
Source: arXiv:2407.00021 source file (2024-10-25)
Supplement: Supplementary file 1 [file errata.tex]

Presented below is the rectification for Figure~5. Regrettably, an error exists in Figure~5 within Section~5.2. The curve associated with our method has been inaccurately plotted. For the corrected curve related to our method, kindly consider Figure~\ref{fig:rd_curve_corrected}. 

\begin{figure}[h!]
    \centering
     \begin{subfigure}[b]{0.47\textwidth}
         \centering
         \includegraphics[width=1\textwidth]{Figs/ours_ntc_astc_2k_rd_corrected.pdf}
         % \caption{}
         \label{fig:rd_curve_psnr}
     \end{subfigure}
     \hspace{-0cm}
     \begin{subfigure}[b]{0.485\textwidth}
         \centering
         \includegraphics[width=1\textwidth]{Figs/ours_ntc_astc_2k_rd_ssim_corrected.pdf}
         % \caption{}
         \label{fig:rd_curve_ssim}
     \end{subfigure}
     % \vspace{-0.2in}
    \caption{Comparison with the state-of-the-art method NTC~\cite{Vaidyanathan2023}.}
    \label{fig:rd_curve_corrected}
\end{figure}
